# Supplementary material for: Coupled skyrmion sublattices in Cu2OSeO3
Source: arXiv:1402.2947 source file (2014-04-19)
Supplement: Supplementary file 1 [file skyrmion_v6_supplemental.tex]

\setcounter{figure}{0}
\makeatletter

\begin{center}
Supplementary Material for\\ ``Coupled skyrmion sublattices in Cu$_{2}$OSeO$_{3}$''
\end{center}

\section{Skyrmion Sublattice Rotation}

The magnetic field dependence of the the skyrmion sublattice rotation implies an interaction between a magnetization along the field direction resulting from canting and a long range modulation of the ferrimagnetism.  We discuss this interaction using a simplified local Hamiltonian and in the context of a Ginzburg-Landau (GL) free energy expansion.

A full local Hamiltonian would need to account for all exchange and DM interactions between the unit cell copper spins \cite{Yang, Chizhikov}.  For a more qualitative description, we consider a simplified hamiltonian, treating the unit cell spins as effective on-site magnetizations of the Cu-I and Cu-II sublattices with effective long-range exchange and Dzyaloshinskii-Moriya (DM) interactions.

\begin{equation}
\label{eq:Heff}
H = - \sum_{i,j} J_{I} \left( m^{(I)}_{i} \cdot m^{(I)}_{j} \right) + J_{II} \left( m^{(II)}_{i} \cdot m^{(II)}_{j} \right) - K \left( m^{I}_{i} \cdot m^{II}_{i} \right) + D_{I} \cdot \left( m^{I}_{i} \times m^{I}_{j}  \right) + D_{II} \cdot \left( m^{II}_{i} \times m^{II}_{j} \right) + B \cdot \left( m^{I}_{i} +  m^{II}_{i}  \right)
\end{equation}

The result of the application of a magnetic field $B$ is to cant the magnetization vectors toward the field direction.  In this simplified model, canting of individual spins in the unit cell can also lead to differential changes in the length of the vectors $m^{I}$ and $m^{II}$, effectively altering the local ferrimagnetism. 

In the case where the on-site antiferromagnetic interaction dominates, a single spiral will form along the direction of the net anisotropic DM exchange, i.e. the spins align in planes perpendicular to $D$.  This is consistent with what we observe experimentally in the helical and conical phases.  A relative rotation of one sublattice is a local tilt of one spin plane relative to the other.  Adding a term to the Hamiltonian with symmetry $M \times \delta M_{z}\left( B \right)$ gives a rotation dependent on the applied field, where $\delta M_{z}\left( B \right)$ is the change in magnetization resulting from spin canting.  This term will change the direction of the net anisotropic exchange without significant changes to the amplitude of the wave vector.  This term has a symmetry similar to that of the spin-orbit coupling driven DM interactions, and can act preferentially on one sublattice either through differences in the magnitude of the canted moment or through differences in the coupling between the canted moment and spiral spin-ordering.  We note that there are multiple DM interactions within the unit cell and the exchange is frustrated.  Hence a single DM vector is unlikely to describe all modes of the system.

In the conical state, this term adds an extra anistropy and changes the symmetry.  In the skyrmion phase, the change in q is equivalent to a sublattice rotation; in this phase the rotational symmetry is already broken by the preferred handedness of the skyrmion, set by the sign of the DM term.

\section{Magnetic Free Energy}

The interaction between the canting and long-range ferrimagnetic modulation can be described in the GL expansion by adding higher-order terms related the spin-orbit coupling (SOC) \cite{SOC_paper}.  We consider the following free energy, assuming that the system remains in the skyrmion phase with six-fold symmetry, therefore ignoring the $M^2$ and $M^4$ and keeping only the terms that affect the wave vector and symmetry of the skyrmion.

\begin{equation}
\label{eq:EGL}
F = (J/2)(\nabla M_{i})^2 + D M \cdot \left( \nabla \times M \right) + K \left( M_{I} \cdot M_{II} \right) - B \cdot M + A \sum_{i} M_{i} \cdot \left( \nabla M_{i} \right)
\end{equation}

Here, M represents the total magnetization of the two sublattices, $M = M_{I} + M_{II}$, and we've added a term with coefficient $K$ to represent the on-site antiferromagnetic coupling between the sublattices.  The term with coefficient $A$ represents a SOC term that favors a modulation of the total magnetization.   We ignore the next highest order term in the SOC, included in \cite{SOC_paper} to bound the total magnetization, as this is bound in our case by fixing the sublattice magnetizations.  Canting within the Cu$_{2}$OSeO$_{3}$ unit cell provides the necessary degrees of freedom for the system to remain in the skyrmion phase, while still minimizing this free energy term by modulating the magnetization.  The magnetic field dependence of the rotation results from the development of a magnetization $\delta M_{z}$, which changes the energy of the $A$ term through $\delta M_{z} \cdot \left( \nabla M_{z} \right)$ and lowers the energy for modulations of $M_{z}$.

To analyze the free energy, we numerically integrate the free energy terms for different rotation angles and canted magnetic moments.  The angular dependence of the K, A, and B terms are shown in figure \ref{fig:S1}.  The B term of the free energy (Fig. \ref{fig:S1}(a) naturally has a strong dependence on the canted moment, with a weak dependence on the relative rotation of the skyrmion lattices.  The K term (Fig. \ref{fig:S1}(c)), and similarly the J and D terms, has a small dependence on the canted moment but depends strongly on the rotation angle.  The SOC term (Fig. \ref{fig:S1}(b)) couples the canted moment and rotation angle, favoring a rotation away from $\phi = 0$, with an energy scale sensitve to $\delta M_{z}$.

\begin{figure*}
\includegraphics[width=6in]{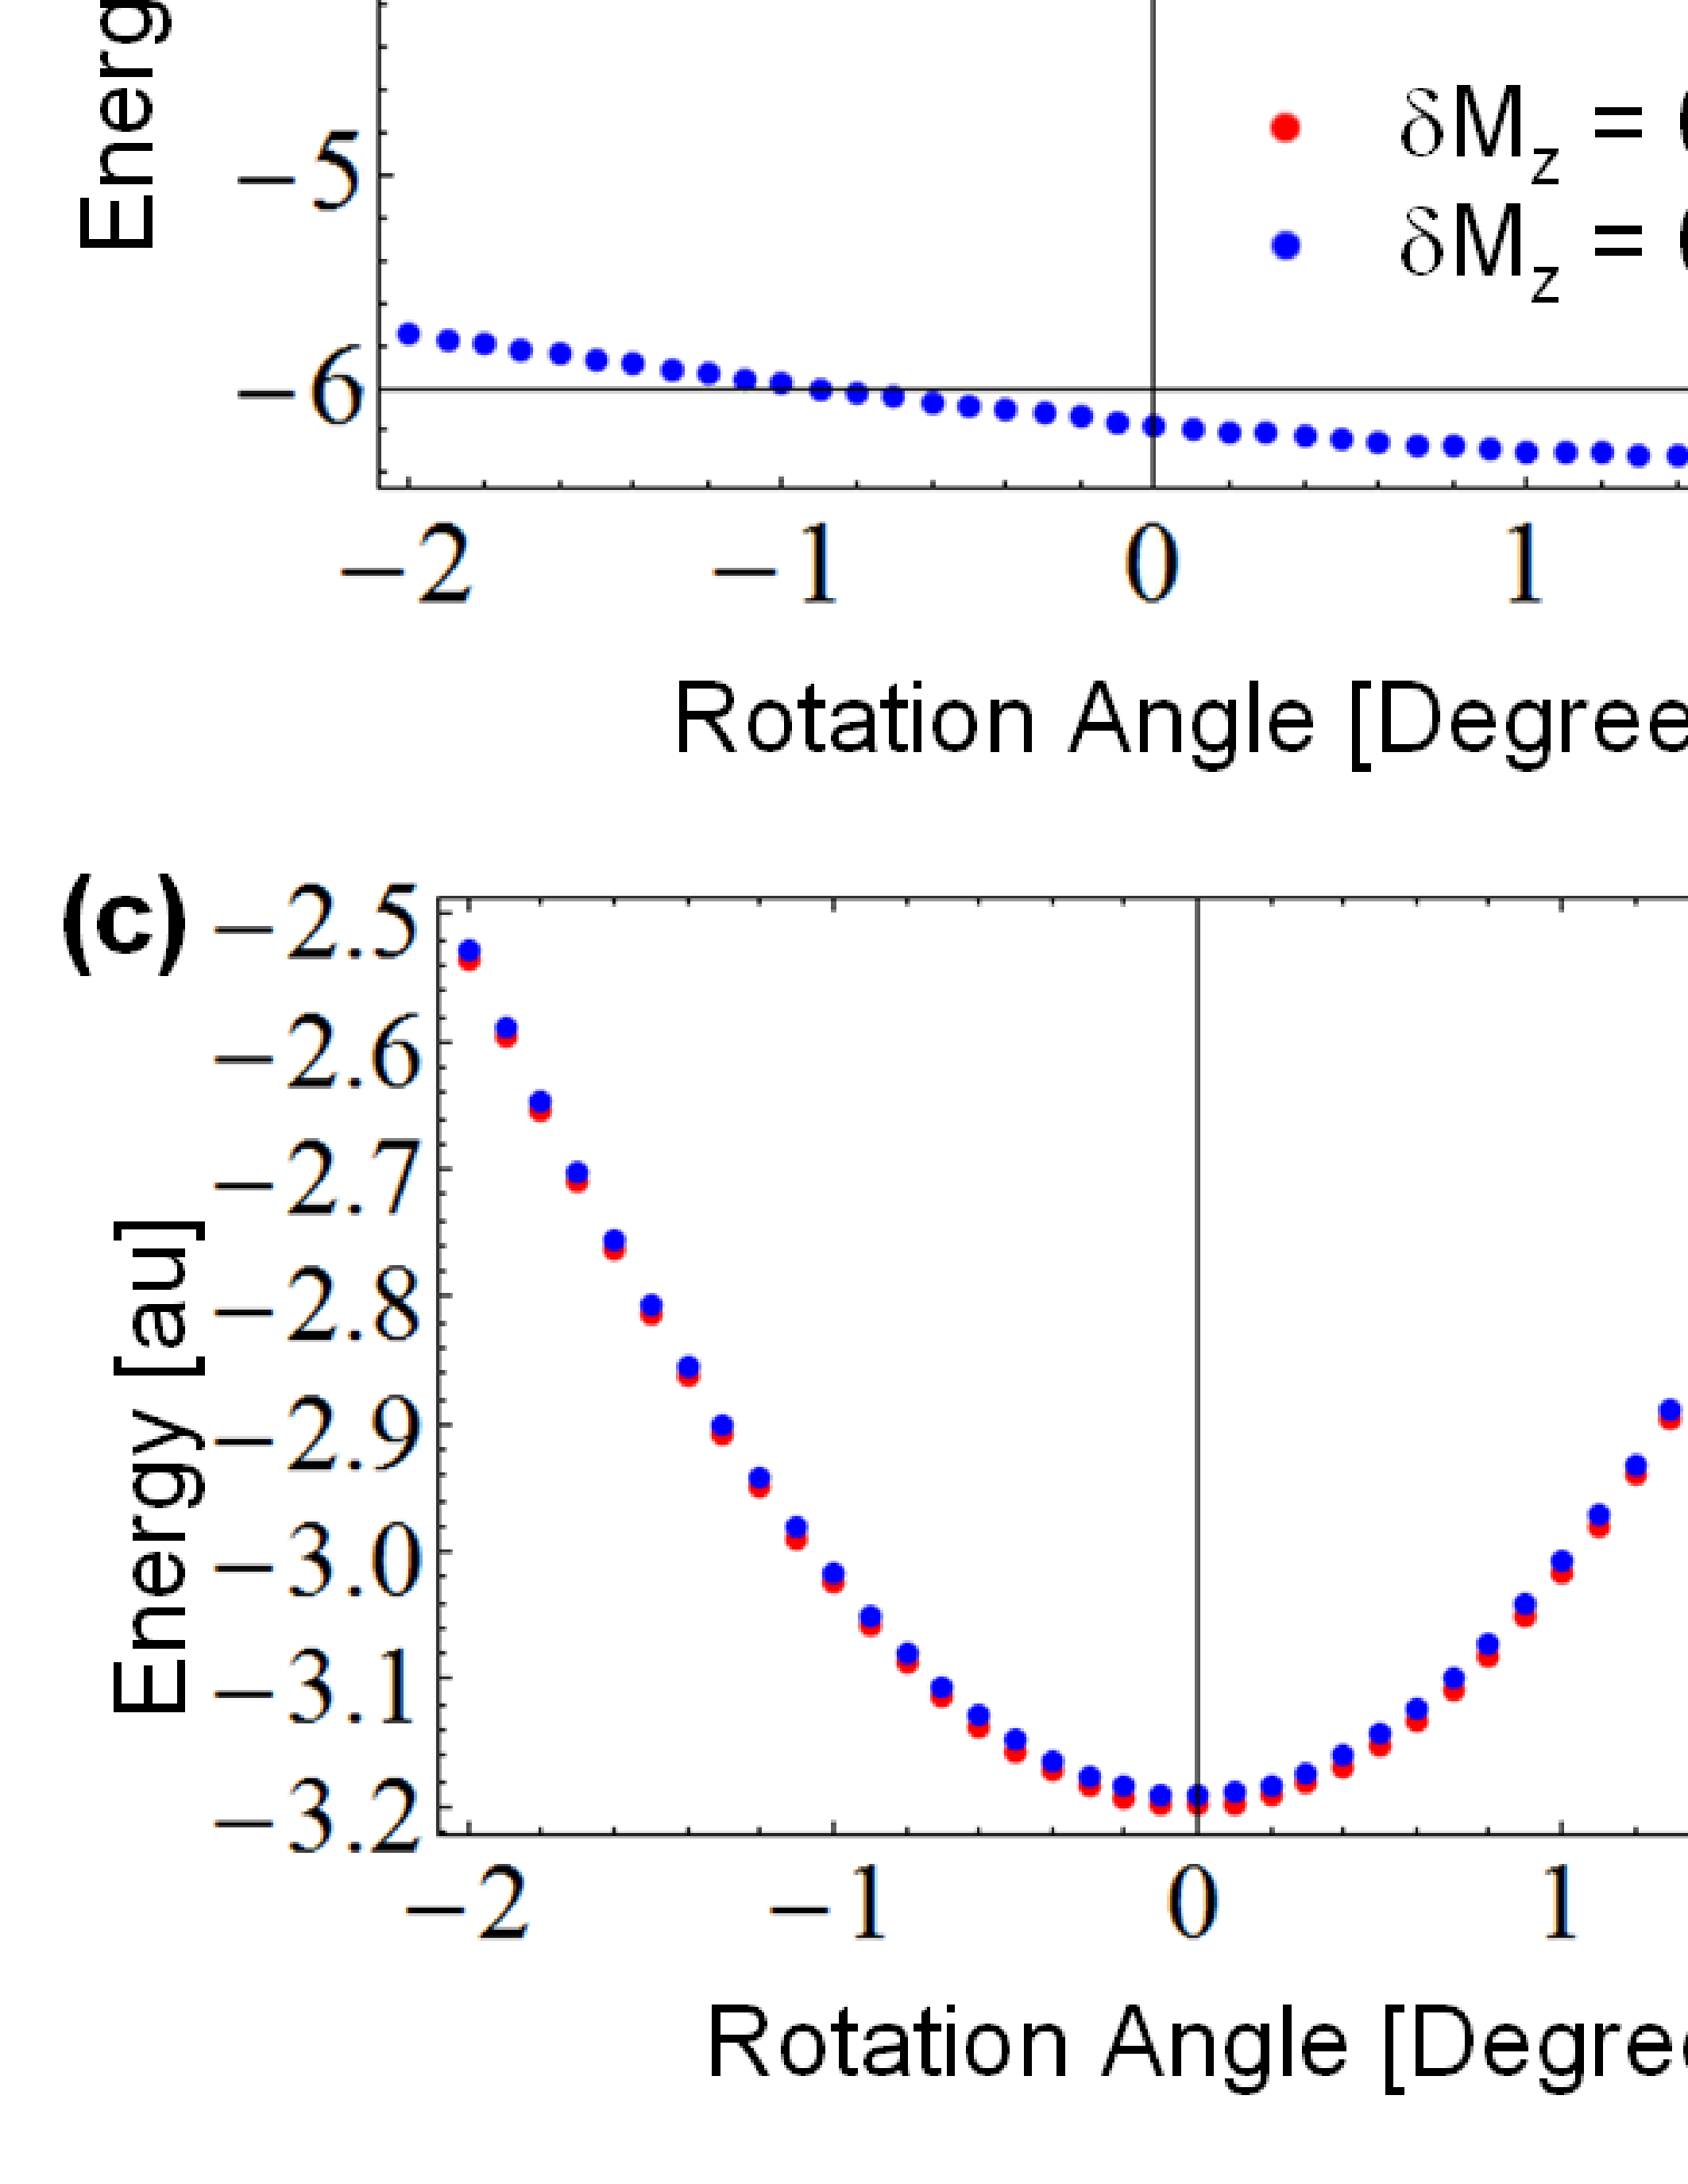}
\caption{Angular depedence of (a) The $B \cdot M$ term. (b) The $A \sum_{i} M_{i} \cdot \left( \nabla M_{i} \right)$ term.  (c) The $K \left( M_{I} \cdot M_{II} \right)$ term.  Note the scaling is arbitrary.  Red and blue dots correspond to a uniform $\delta M_{Z}$ of 0.05 (red) and 0.1 (blue).}
\label{fig:S1}
\end{figure*}
